# Supplementary material for: Hyperspectral Image Analysis in Single-Modal and Multimodal setting using Deep Learning Techniques
Source: arXiv:2403.01546 source file (2024-03-03)
Supplement: Supplementary file 1 [file Appendix_I.tex]

\chapter{Measurement system}

\section{Introduction}
Here we go... decomposition methodologies available in the literature. Moreover, it also contains algorithms for snowpack parameters estimation from single, dual and full- polarimetric SAR data. 

\section{Functionalities}
Many pre and post-processing steps are included along with the snowpack parameter estimation algorithms in this HimSAR toolbox.
