# Supplementary material for: Hyperspectral Image Analysis in Single-Modal and Multimodal setting using Deep Learning Techniques
Source: arXiv:2403.01546 source file (2024-03-03)
Supplement: Supplementary file 2 [file Appendix_II.tex]

\chapter{Measurements Techniques}
Field campaigns were conducted in month of February over the study area.
